# Supplementary material for: Sequential Signal Mixing Aggregation for Message Passing Graph Neural Networks
Source: arXiv:2409.19414 source file (2024-09-28)
Supplement: Supplementary file 1 [file 3o_proof_wasserstein_thm.tex]

\section{Proof of \cref{thm:wasserstein}} \label{appendix:wasserstein_thm}

Let $\overline{X},\overline{Y}$ be two multisets of $d$ dimensional vectors of size $n$.

We first prove the following fact:

\begin{equation} \label{eq:helper_lemma}
    \forall t,z \in \C \text{ with } |t|=|z|=1: |p_{\overline{X}}(t,z) - p_{\overline{Y}}(t,z)| \leq n(1+\delta)^{n-1} \cdot \W_1(\overline{X}, \overline{Y})
\end{equation}

Let $\pi \in S_n$ be the permutation that minimizes $\frac{1}{n}\sum_{i=1}^n \norm{X_i - Y_{\pi(i)}}$.
The key idea of the proof is to define the following hybrid polynomials:

\begin{equation}
    p_i(t,z) := (t-q_{X_1}(z))\cdot...\cdot(t-q_{X_i}(z))\cdot(t-q_{Y_{\pi(i+1)}}(z))\cdot...\cdot(t-q_{Y_{\pi(n)}}(z))
\end{equation}

We have that $p_0(t,z) = p_{\overline{Y}}(t,z)$ and $p_n(t,z) = p_{\overline{X}}(t,z)$. 
We can hence rewrite the following:

\begin{align}
    & 	\Bigg | p_{\overline{X}}(t,z) - p_{\overline{Y}}(t,z) \Bigg |  = \\
    & 	\Bigg | \sum_{i=1}^n (p_i(t,z) - p_{i-1}(t,z)) 	       \Bigg | \leq \\
    & \sum_{i=1}^n 	\Bigg | p_i(t,z) - p_{i-1}(t,z) \Bigg |  = \\
    & \sum_{i=1}^n 	\Bigg | (t-q_{X_1}(z))\cdot...\cdot(t-q_{X_i}(z))\cdot(t-q_{Y_{\pi(i+1)}}(z))\cdot...\cdot(t-q_{Y_{\pi(n)}}(z)) - \\
    & (t-q_{X_1}(z))\cdot...\cdot(t-q_{X_{i-1}}(z))\cdot(t-q_{Y_{\pi(i)}}(z))\cdot...\cdot(t-q_{Y_{\pi(n)}}(z)) \Bigg | = \\
    & \sum_{i=1}^n 	\biggl\{ \prod_{j<i} |t-q_{X_j}(z)| \biggr\} 
                    \cdot \Bigg | q_{Y_{\pi(i)}}(z) - q_{X_i}(z) \Bigg | \cdot
                    \biggl\{ \prod_{j>i} |t-q_{Y_{\pi(j)}}(z)| \biggr\} 
\end{align}

For the middle term we have:

\begin{align}
    & 	\Bigg | q_{X_i}(z) - q_{Y_{\pi(i)}}(z) \Bigg |  = 
        \Bigg | \sum_{k=0}^{d-1} (X_{ik} - Y_{\pi(i)k})z^k \Bigg | \leq \\
    &    \sum_{k=0}^{d-1} | X_{ik} - Y_{\pi(i)k} | \cdot |z|^k = 
        \sum_{k=0}^{d-1} | X_{ik} - Y_{\pi(i)k} | = 
        \norm{X_i - Y_{\pi(i)}}
\end{align}

For the other terms (w.l.o.g in the first group), we have:

\begin{align}
     & | t-q_{X_j}(z) | \leq
       |t| + |q_{X_j}(z)| =
       1 + \Bigg | \sum_{k=0}^{d-1} X_{jk}z^k \Bigg | \leq 
       1 + \sum_{k=0}^{d-1} |X_{jk}| \cdot |z|^k = 
       1 + \sum_{k=0}^{d-1} |X_{jk}| = 1 + \norm{X_j} \leq 1 + \delta
\end{align}

Plugging in all the terms, we get:

\begin{equation} 
    \Bigg | p_{\overline{X}}(t,z) - p_{\overline{Y}}(t,z) \Bigg |  \leq 
    \sum_{i=1}^n (1+\delta)^{n-1} \norm{X_i - Y_{\pi(i)}} = n(1+\delta)^{n-1} \cdot \W_1(\overline{X}, \overline{Y})
\end{equation} 

Now, we have that:

\begin{align}
    & \biggl | [f_{conv}(\overline{X}) - f_{conv}(\overline{Y})]_{k,l} \biggr | = \\ 
    & \frac{1}{n+1} \cdot \frac{1}{1+\tau} 
    \Biggl | \sum_{s=0}^n \sum_{b=0}^{\tau} p_{\overline{X}}(e^{-\frac{2 \pi i}{n+1}s},e^{-\frac{2 \pi i}{\tau+1}b}) 
    e^{\frac{2 \pi i}{n+1}k s} e^{\frac{2 \pi i}{\tau+1}\ell b} - 
    \sum_{s=0}^n \sum_{b=0}^{\tau} p_{\overline{Y}}(e^{-\frac{2 \pi i}{n+1}s},e^{-\frac{2 \pi i}{\tau+1}b}) 
    e^{\frac{2 \pi i}{n+1}k s} e^{\frac{2 \pi i}{\tau+1}\ell b} \Biggr | \leq \\
    & \frac{1}{n+1} \cdot \frac{1}{1+\tau} 
     \sum_{s=0}^n \sum_{b=0}^{\tau} 
     \biggl | p_{\overline{X}}(e^{-\frac{2 \pi i}{n+1}s},e^{-\frac{2 \pi i}{\tau+1}b}) -
     p_{\overline{Y}}(e^{-\frac{2 \pi i}{n+1}s},e^{-\frac{2 \pi i}{\tau+1}b}) \biggr | \cdot
    \biggl | e^{\frac{2 \pi i}{n+1}k s} \biggr | \cdot 
    \biggl | e^{\frac{2 \pi i}{\tau+1}\ell b} \biggr | \leq \\
    & \frac{1}{n+1} \cdot \frac{1}{1+\tau} 
     \sum_{s=0}^n \sum_{b=0}^{\tau} 
     n(1+\delta)^{n-1} \cdot \W_1(\overline{X}, \overline{Y}) \cdot
    1 \cdot 
    1 = n(1+\delta)^{n-1} \cdot \W_1(\overline{X}, \overline{Y})
\end{align}

Where in the last inequality we used \cref{eq:helper_lemma} with $t=e^{-\frac{2 \pi i}{n+1}s}$ and $z=e^{-\frac{2 \pi i}{\tau+1}b}$.
Summing over all $k,\ell$ we finally get:

\begin{equation}
\norm{f_{conv}(\overline{X}) - f_{conv}(\overline{Y})} = 
\sum_{k=0}^n \sum_{\ell=0}^{\tau} | [f_{conv}(\overline{X}) - f_{conv}(\overline{Y})]_{k,l} | \leq
(n+1)^3d(1+\delta)^{n-1} \cdot \W_1(\overline{X}, \overline{Y})
\end{equation}

So setting $C(n,d,\delta) := (n+1)^3d(1+\delta)^{n-1}$ concludes the theorem. \qed
