# Supplementary material for: Sequential Signal Mixing Aggregation for Message Passing Graph Neural Networks
Source: arXiv:2409.19414 source file (2024-09-28)
Supplement: Supplementary file 2 [file 7_normalization_factor.tex]

\section{The normalization in \aggname} \label{appendix:normalization_factor}

Here, we show that our normalization bounds the magnitude of the output of our aggregation. Let $A_{max} = \max_{i \in \mathcal{N}_{{in}_y}} \left( \left| \mathcal{F} \left( A(\vec{h_i}) \right) \right| \right)$ as the maximum amplitude of the elements multiplied by the Fourier transformation in \cref{eq:circular_equation_impl}.

\begin{align}
    \left| \left( \prod\limits_{i \in \mathcal{N}_{{in}_y}} \mathcal{F} \left( \mathcal{A} \left( \vec{h_i} \right) \right) \right)^{\frac{1}{|\mathcal{N}_{{in}_y}|}} \right| \leq \left( \prod\limits_{i \in \mathcal{N}_{{in}_y}} \left| \mathcal{F} \left( \mathcal{A} \left( \vec{h_i} \right) \right) \right| \right)^{\frac{1}{|\mathcal{N}_{{in}_y}|}} \leq \left( \prod\limits_{i \in \mathcal{N}_{{in}_y}} A_{max} \right)^{\frac{1}{|\mathcal{N}_{{in}_y}|}} = A_{max}
\end{align}
